# Supplementary material for: SFDM: Robust Decomposition of Geometry and Reflectance for Realistic Face Rendering from Sparse-view Images
Source: arXiv:2312.06085 source file (2025-03-15)
Supplement: Supplementary file 1 [file 7_supp.tex]

\section{Overview}

This supplementary material provides additional results and analysis that support the methodology of our main text.
We provide more details on the implementation of our method in Sec.~\ref{sec:implementation}. 
To validate the effectiveness and robustness of our proposed method, we give additional results for subjects with divergent characteristics and experiments conducted on \textit{H3DS}~\cite{ramon2021h3d} in Sec.~\ref{sec:generalization}. 
In addition, we analyze the experimental results in detail in Sec.~\ref{sec:analysis}, including quantitative and qualitative metrics comparisons with other work. In Sec.~\ref{sec:single}, we discuss the relationship between our task and single-view reconstructions, highlighting the advantages and limitations of each. Sec.~\ref{sec:ethnic} contemplates the potential negative impact of our work and our responsibility to human subjects. Extensive visualization results can be found in Sec.~\ref{sec:additional_results}.

% \section{Geometry Decomposition from Neural Fields}

% Leveraging multi-view images, NeRF~\cite{mildenhall2021nerf} has excelled in generating high-quality novel view images~\cite{barron2021mip,muller2022instant,verbin2022ref}, thanks to its implicit 3D representation that enhances understanding of 3D spaces. However, its implicit nature complicates interpretability, editing, and manipulation. Transitioning to explicit 3D forms like meshes is vital for clearer geometry decomposition, but direct mesh extraction from NeRF's density often falls short. Addressing this, VolSDF~\cite{yariv2021volume} and NeuS~\cite{wang2021neus} integrate Signed Distance Fields (SDF) into the volume rendering, improving geometry reconstruction and enabling obtaining detailed 3D meshes.

% 3) analysis about the quantitative and qualitative comparison between different methods in Sec.~\ref{sec:discussion}, delving into the reasons behind the results; and 4) extensive results visualization in Sec.~\ref{sec:additional_results}, providing a more comprehensive comparison between different methods.

\begin{figure}[htbp]
    \centering
    \includegraphics[width=0.95\linewidth]{figs/supp/method_cmp.jpg}
    \\
    \hspace{-30pt}\makebox[0.32\linewidth]{\scriptsize{(a) 3D Reconstruction}\hspace{0pt}}
    \makebox[0.32\linewidth]{\hspace{-5pt}\scriptsize(b) BRDF Decomposition}\hspace{-20pt}
    \makebox[0.32\linewidth]{\hspace{20pt}\scriptsize(c) SFDM}
    \vspace{-5pt}
    \caption{\textbf{Overview of different frameworks.} \textbf{(a)} Framework like VolSDF~\cite{yariv2021volume} accomplishes 3D reconstruction from dense images but does not decompose radiance-related factors. \textbf{(b)} Framework like NerFactor~\cite{zhang2021nerfactor} introduces physically based rendering (PBR) to simulate real-world lighting. \textbf{(c)} We propose a novel geometry and reflectance decomposition framework for 3D face reconstruction from sparse views.}
    \label{fig:overview}
\end{figure}

\section{Implementation details}
\label{sec:implementation}

\textbf{Network Architecture.} In Stage 1, we aim to learn a general facial template with both geometry and reflectance attributes. For the geometry template, we slightly modify the identity mini-nets and template mini-nets of ImFace~\cite{zheng2022imface}. Specifically, we introduce two additional MLPs as feature extraction branches for each part, together with the mini-nets, forming our deformation net $F_{\text{dfm}}$ and template net $T_{\text{geo}}$, respectively. Regarding the reflectance template $T_{\text{rfl}}$, we utilize an 8-layer MLP with 256 dimensions in each layer, and the BRDF offset module $F_{\text{ofs}}$ employs the same architecture. The PBR module uses an MLP consisting of four layers, each with 128 dimensions, to compute the BRDF look-up-textures $B_{0}$ and $B_{1}$. For the albedo gradient predictor $\mathcal{G}$, we also employ a four-layer MLP with 128 dimensions.
% Within the PBR module, an MLP comprising 4 layers with 128 dimensions is employed to calculate the BRDF look-up-textures B0 and B1.

\begin{figure}[htbp]
    \centering
    \includegraphics[width=0.65\linewidth]{figs/supp/ss_v2.pdf}
    \caption{The network architecture of subsurface scattering offset.}
    \label{fig:scatter-net}
\end{figure}

In Stage 2, we introduce two additional modules: the displacement net $F_{\text{dis}}$ and the subsurface scattering offset net $F_{\text{ss}}$. The displacement net is composed of a 4-layer MLP, with each layer having 256 dimensions. To capture high-frequency geometric details, we incorporate a positional encoding of 8 frequencies. The architecture of the subsurface scattering offset module is illustrated in Fig.~\ref{fig:scatter-net}. At first, we use a 4-layer MLP (Param-net) to obtain the scattering parameters $\mathbf{f}^{\mathbf{x}}_{\text{sp}}$ and a vector $\mathcal{E}(\mathbf{x})$ indicating the light integration region. Subsequently, we utilize two branches to integrate light and scattering reflectance. In the light integration branch, we initially compress the Spherical Harmonics (SH) weights into an ambient light embedding $ \mathbf{z}_{\text{lgt}}$ by using a linear layer. 
Afterwards, we utilize a light integration network $\hat{L}_{\text{i}}$ to obtain the light intensity of a small region on the surface as $\hat{L}_{\text{i} }(\textbf{x}, \mathbf{z}_\text{lgt}, \mathcal{E}(\mathbf{x} ))$, where $\textbf{x}\in\mathbb{R}^3$ are the coordinates. For scattering reflectance, the scattering reflectance integration network $\hat{F}_{\text{sp}}$ integrates the scattering reflectance based on the scattering parameters $\mathbf{f}^{\mathbf{x}}_{\text{sp}}$ and coordinates $\textbf{x}$, resulting in the output of integrated reflectance. Both $\hat{L}_{\text{i}}$ and $\hat{F}_{\text{sp}}$ comprise a 4-layer MLP. We use sine activation to allow the model to more effectively handle Gaussian curves in scattering profiles. Finally, the 3-dimensional integrated light and scattering reflectance are multiplied to produce the offset term for diffuse components.

\noindent\textbf{Volume rendering.} 
Following most previous work~\cite{mildenhall2021nerf}, we calculate the color by integrating the radiance $L_{\text{o}}$ and density $\sigma\in\mathbb{R}$ along the ray $\mathbf{r}$ as:
\begin{equation}\label{eq:volume-rendering}
    \mathbf{C}(\mathbf{r})=\int_{t'}^{t''} L_{\text{o}}(\mathbf{x}(t), \boldsymbol{\omega}_{\text{o}}) \sigma(t) T(t)\,\, \mathrm{d}t,
\end{equation}
where $\mathbf{x}(t)$ represents the coordinates of a point in the ray, with $t'$ and $t''$ as the starting and ending points along the ray, respectively. $T(t)=\exp (-\int_{t_{n}}^{t'} \sigma(t)\,\, \text{d} t)$, which can be considered as the radiance attenuation rate caused by hitting particles along the ray.

%In stage 1, for the geometry template, we use ImFace to implement the deformation net and template net, and add two linear layers to extract the feature vectors for the deformation net and template net respectively. For the reflectance template, we use 8 layers of MLP, each layer 256 dimensions, which is of the same structure as the offset net. In the PBR module, we use a small MLP with 4 layers of 128 dimensions to calculate B0 and B1.

%In stage 2, for displacement net, we use 4 layers of MLP, each 256 dimensions and we use a positional embedding of 8 to capture more high-frequency details. For the subsurface scattering offset module, the architecture is shown in figure. First, we use a scatter profile network to output the scatter parameters and a region indicator. Then, we use two branches to integrate light and reflectance. For light integration, we first use a linear layer to compress the SH weights to an ambient light embedding. Next, we input the light embedding, coordinates, and region indicator to the light integration network, and then output an integrated light intensity. For reflectance integration, we input the scattering profile embedding and coordinates to the reflectance integration net, and output integrated reflectance. Finally, we multiply the integrated light and reflectance and get the offset term for diffuse.

% To ensure the face template consists of the majority of facial features, we select the expression "grin" to capture additional details in the mouth.
\noindent\textbf{Data preprocessing.} We mainly use the \textit{Facescape}~\cite{yang2020facescape} dataset, which contains 359 subjects in 20 different expressions. For each subject, \textit{Facescape} has over 50 multi-view images, along with corresponding camera parameters and scanned meshes. We select 3, 5, and 10 frontal views for training, and around 10 views for testing. 
Before training the model, we first preprocess the images and camera parameters. Adopting the preprocessing approach of NeuFace~\cite{zheng2023neuface} and ImFace~\cite{zheng2022imface}, we crop the facial region from the \textit{Facescape} head mesh and align the cropped mesh within the [-1, 1] range. 
This cropped mesh is also used as ground truth for evaluating geometry accuracy.
For camera parameters, we adjust the original \textit{Facescape} camera settings to correspond with the mesh processing operations. Regarding the images, using the updated camera parameters, we can render the corresponding face masks, which then allows us to extract the facial regions from the original images.

\noindent\textbf{Training details.} During training, we use 10 subjects, each with 10 views images from \textit{Facescape} to train the facial template in Stage 1. 
We tested 3, 6, 10, and 15 subjects for template training, finding that performance saturates between 6 and 10 subjects.
We employ the pre-trained ImFace model to initialize the geometry template. To promote stable template learning, we apply a weight of 0.02 to the learning rate for template optimization, which effectively avoids severe variation. The total loss function for Stage 1 is:
\begin{equation}
    \begin{split}
\mathcal{L}_{\text{st1}}=&\lambda_1\mathcal{L}_{\text{col} }+\lambda_2\mathcal{L}_{\text{eik} }+\lambda_3\mathcal{L}_{\text{light} }+\lambda_4\mathcal{L}_{\text{spec}}+\lambda_5\mathcal{L}_{\text{ofs}} \\ &+\lambda_6\mathcal{L}_{\text{code}}+\lambda_7\mathcal{L}_{\mathcal{G}},
\end{split}
\end{equation}
where $\lambda_{1}, \cdots, \lambda_{7}$ are $1$, $1e^{-1}$, $5e^{-3}$, $1.5e^{-2}$, $1e^{-3}$, $500$, and $5e^{-3}$, respectively. 

%In stage 2, we only choose subjects that never occur in stage 1 as our training data. For the 3-view setting, we mainly choose one frontal photo and two profile photos. We use a set of learnable parameters to adjust the contribution of each BRDF parameter from the reflectance template. Specifically, we initialize the weight of each albedo channel by 0.4, and others by 0.9, due to the large variation of albedo. During training, the learning rate of template optimization is weighted by a small weight of 0.02, which maintains the majority of template information and is able to slightly modify the template parameters to be more suitable in stage 2. There are two new losses in stage 2, and we assign a weight for each one:

In Stage 2, we select subjects that are not used during Stage 1. We mainly select one frontal image and two profile images in the 3-view setting, so as to capture the most comprehensive facial information of an individual. To adjust the contribution of each BRDF parameter from the reflectance template, we employ a set of learnable parameters $\mathbf{W}(\mathbf{x})$. Specifically, we initialize the weight of each albedo channel in $\mathbf{w}_{\text{a}}$ to 0.4, while setting others to 0.9 due to the substantial variation in albedo.
During the second training stage, we apply a weight of 0.02 to the learning rate for template optimization. This approach ensures that the majority of template information is retained, while still allowing for slight modifications to enhance the suitability of template parameters in Stage 2. The loss function for Stage 2 is based on Stage 1 with two additional items:
\begin{equation}
\mathcal{L}_{\text{st2}}=\mathcal{L}_{\text{st1}}+\lambda_8\mathcal{L}_{\text{dis}}+\lambda_9\mathcal{L}_{\text{ss} },
\end{equation}
where $\lambda_8=1e^{-3}$ and $\lambda_9=2e^{-3}$. Since the albedo gradient predictor $\mathcal{G}$ is not trained during Stage 2, we set $\lambda_7$ to 0.

%As we mainly focus on decomposition accuracy, we don't implement acceleration techniques such as hash encoding and plenoctree. We train stage 1 using 4 V100s for 20 hours with a mini-batch of 2048 rays. We train stage 2 on 5 views for 2.5 hours.

We conducted our training procedure on Tesla V100 GPUs. In Stage 1, we utilized 4 GPUs for approximately 20 hours, using a mini-batch size of 2048 rays. For Stage 2, we employed 2 GPUs with 3, 5, and 10 views, with each training session lasting around 2, 2.5, and 5 hours respectively. In the future, we plan to explore acceleration techniques such as hash encoding~\cite{muller2022instant} and Plenoctree~\cite{yu2021plenoctrees} to enhance the efficiency of the decomposition and reconstruction processes.

\noindent\textbf{Testing details.} During testing, we apply calibration on all methods to mitigate the exposure differences as NeuFace~\cite{zheng2023neuface}. This process helps eliminate the overall color disparities between the rendered images and the ground truth images caused by unknown illumination or exposure conditions. For example, in Fig.~\ref{fig:3view-sub12}, the diffuse prediction of NeuFace appears yellowish, potentially due to a false assumption about the light being yellow. To minimize the impact of such erroneous assumptions, the calibration aligns the ground truth image by employing a $3\times3$ matrix on the radiance values.

In scenarios involving relighting, we convert the environment maps to SH weights following~\cite{chen2020neural}. For specular editing, we adjust the specular intensity parameter in $b_{\text{s}}$ to control the shininess of faces.

In the reflectance decomposition analysis (Sec. 5.4 of the main text), we utilize RefMM~\cite{han2023learning} to fit and generate pseudo-reflectance ground truth for all test images of five subjects. Subsequently, we calculate the SSIM values for the diffuse and specular results of each subject under the 3, 5, and 10 view settings.

\begin{figure}[htbp]
    \centering
    \makebox[0.02\linewidth]{\rotatebox{90}{\hspace{15pt}\footnotesize 212 Grin}}\hspace{5pt}
    \includegraphics[width=0.15\linewidth]{figs/supp/expression/212_16/212_16_render.pdf}\hspace{5pt}
    \includegraphics[width=0.15\linewidth]{figs/supp/expression/212_16/212_16_normal.pdf}\hspace{5pt}
    \includegraphics[width=0.15\linewidth]{figs/supp/expression/212_16/212_16_diffuse.pdf}\hspace{5pt}
    \includegraphics[width=0.15\linewidth]{figs/supp/expression/212_16/212_16_spec.pdf}
    \\
    \makebox[0.02\linewidth]{\rotatebox{90}{\hspace{12pt}\footnotesize 212 Smile}}\hspace{5pt}
    \includegraphics[width=0.15\linewidth]{figs/supp/expression/212_2/212_2_render.pdf}\hspace{5pt}
    \includegraphics[width=0.15\linewidth]{figs/supp/expression/212_2/212_2_normal.pdf}\hspace{5pt}
    \includegraphics[width=0.15\linewidth]{figs/supp/expression/212_2/212_2_diffuse.pdf}\hspace{5pt}
    \includegraphics[width=0.15\linewidth]{figs/supp/expression/212_2/212_2_spec.pdf}
    \\
    \makebox[0.02\linewidth]{\rotatebox{90}{\hspace{15pt}\footnotesize 344 Grin}}\hspace{5pt}
    \includegraphics[width=0.15\linewidth]{figs/supp/expression/344_16/render.pdf}\hspace{5pt}
    \includegraphics[width=0.15\linewidth]{figs/supp/expression/344_16/normal.pdf}\hspace{5pt}
    \includegraphics[width=0.15\linewidth]{figs/supp/expression/344_16/diffuse.pdf}\hspace{5pt}
    \includegraphics[width=0.15\linewidth]{figs/supp/expression/344_16/spec.pdf}
    \\
    \makebox[0.02\linewidth]{\rotatebox{90}{\hspace{12pt}\footnotesize 344 Angry}}\hspace{5pt}
    \includegraphics[width=0.15\linewidth]{figs/supp/expression/344_4/render.pdf}\hspace{5pt}
    \includegraphics[width=0.15\linewidth]{figs/supp/expression/344_4/normal.pdf}\hspace{5pt}
    \includegraphics[width=0.15\linewidth]{figs/supp/expression/344_4/diffuse.pdf}\hspace{5pt}
    \includegraphics[width=0.15\linewidth]{figs/supp/expression/344_4/spec.pdf}
    \\
    \makebox[0.02\linewidth]{}\hspace{5pt}
    % \makebox[0.15\linewidth]{\footnotesize\textbf{GT}}\hspace{5pt}
    \makebox[0.15\linewidth]{\footnotesize\textbf{Rendering}}\hspace{5pt}
    \makebox[0.15\linewidth]{\footnotesize\textbf{Normal}}\hspace{5pt}
    \makebox[0.15\linewidth]{\footnotesize\textbf{Diffuse}}\hspace{5pt}
    \makebox[0.15\linewidth]{\footnotesize\textbf{Specular}}\hspace{5pt}
    \caption{Results on different expressions.}
    \vspace{-10pt}
    \label{fig:expressions}
\end{figure}

\section{Generalization on out-of-domain data}
\label{sec:generalization}
\noindent\textbf{Different expressions.} During template training, we use randomly selected subjects with the same ``grin'' expression to ensure that the facial template consists of the majority of facial features. 
% In contrast, other expressions may miss certain details due to closed mouths or eyes. Despite this, our method can robustly decompose and reconstruct subjects that have significant differences from the template, such as different expressions, ages, and skin tones.
% To validate the effectiveness of our method for subjects with divergent characteristics from template training data, we test on cases that have large differences from the template, \textit{i.e.}, different expressions, ages, and skin color.
As shown in Fig.~\ref{fig:expressions}, our method exhibits robustness in decomposing subjects with various expressions, since the ``grin'' face contains major elements on human faces (e.g. teeth and eyes).

\noindent\textbf{Divergent characteristics.} Fig.~\ref{fig:age} shows the results of subjects with different skin colors and ages, which have large variations from our facial template. Thanks to our adaptable facial template, enriched with comprehensive human facial priors, SFDM adeptly navigates these challenging scenarios to achieve realistic face reconstructions.

\begin{figure}[htbp]
    % \vspace{-10pt}
    \centering
    \makebox[0.02\linewidth]{\rotatebox{90}{\hspace{15pt}\footnotesize 17 Grin}}\hspace{5pt}
    \includegraphics[width=0.15\linewidth]{figs/supp/age/17/17_render.pdf}\hspace{5pt}
    \includegraphics[width=0.15\linewidth]{figs/supp/age/17/17_normal.pdf}\hspace{5pt}
    \includegraphics[width=0.15\linewidth]{figs/supp/age/17/17_diffuse.pdf}\hspace{5pt}
    \includegraphics[width=0.15\linewidth]{figs/supp/age/17/17_spec.pdf}
    \\
    \makebox[0.02\linewidth]{\rotatebox{90}{\hspace{12pt}\footnotesize 14 Grin}}\hspace{5pt}
    \includegraphics[width=0.15\linewidth]{figs/supp/age/14/14_render.pdf}\hspace{5pt}
    \includegraphics[width=0.15\linewidth]{figs/supp/age/14/14_normal.pdf}\hspace{5pt}
    \includegraphics[width=0.15\linewidth]{figs/supp/age/14/14_diffuse.pdf}\hspace{5pt}
    \includegraphics[width=0.15\linewidth]{figs/supp/age/14/14_spec.pdf}
    \\
    \makebox[0.02\linewidth]{}\hspace{5pt}
    % \makebox[0.15\linewidth]{\footnotesize\textbf{GT}}\hspace{5pt}
    \makebox[0.15\linewidth]{\footnotesize\textbf{Rendering}}\hspace{5pt}
    \makebox[0.15\linewidth]{\footnotesize\textbf{Normal}}\hspace{5pt}
    \makebox[0.15\linewidth]{\footnotesize\textbf{Diffuse}}\hspace{5pt}
    \makebox[0.15\linewidth]{\footnotesize\textbf{Specular}}\hspace{5pt}
    \caption{Results of subjects with large variations of skin colors and ages from the template.}
    % \vspace{-10pt}
    \label{fig:age}
\end{figure}

% \noindent\textbf{H3DS.} To further verify the generalization performance of our method on out-of-domain data, we conducted additional experiments on the H3DS dataset~\cite{ramon2021h3d}. We directly used the facial template trained on \textit{Facescape} for Stage 1, which allowed us to better assess the performance of the facial template on unseen data. Moreover, we conducted an ablation study on the components of Stage 1 to further validate the contribution of our template to the robustness of decomposition. As shown in Fig.~\ref{fig:h3ds}, in the absence of the template and albedo gradient predictor, the model exhibited various degrees of decomposition errors in sparse view scenarios, such as mistakes in the nose area. In contrast, with a complete facial template, despite facing challenges—training a new template on new data, imprecise facial segmentation in H3DS, and significant lighting differences across views (some with flash)—our method was still able to accurately decompose the face. To further enhance the robustness of decomposition results for subjects with significant domain gaps, a more effective approach may involve training the facial template on a more extensive and diverse set of subjects.

\begin{figure}[htbp]
\vspace{-10pt}
\centering
\includegraphics[width=0.18\linewidth]{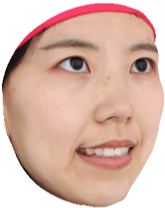}
\includegraphics[width=0.18\linewidth]{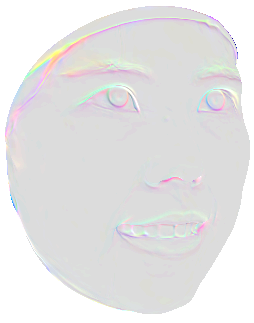}
\makebox[0.1\linewidth]{}
\includegraphics[width=0.18\linewidth]{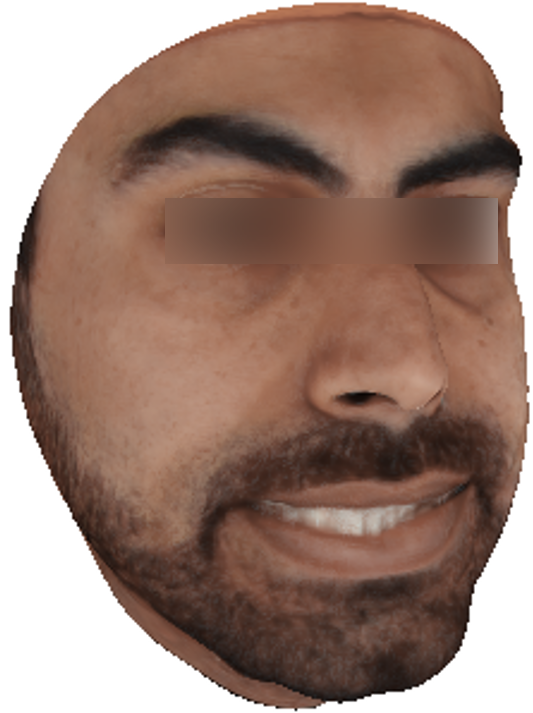}
\includegraphics[width=0.18\linewidth]{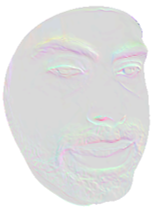}
% \makebox[0.48\linewidth]{\footnotesize \textbf{Image}}
% \makebox[0.48\linewidth]{\footnotesize $\nabla \mathbf{b}_{\text{a}}$}
\caption{\textbf{Albedo gradient visualization.} The albedo gradient can partially outline the sketches of human faces and provide additional guidance for albedo prediction.}
\label{fig:albedo_g}

\end{figure}
\noindent\textbf{H3DS.} To further verify the generalization performance of our method on out-of-domain data, we conduct additional experiments on the \textit{H3DS} dataset~\cite{ramon2021h3d}. We directly use the facial template trained on \textit{Facescape} for Stage 1, which allows us to better assess the performance of the facial template on unseen data. Moreover, we carry out an ablation study on the components of Stage 1 to further validate the contribution of our template to the robustness of decomposition. As shown in Fig.~\ref{fig:h3ds}, in the absence of the template and albedo gradient predictor, the model exhibits various degrees of decomposition errors in sparse view scenarios, such as mistakes in the nose area. In contrast, with a complete facial template, despite facing challenges—without training a new template on new data, imprecise facial segmentation in \textit{H3DS}, and significant lighting differences across views (some with flash)—our method is still able to decompose the face. 
We also visualize the albedo gradient in Fig.~\ref{fig:albedo_g}, which resembles a sketch of the human face. The albedo gradient provides a more generalized representation than the absolute values of albedo, enhancing the model's ability to generalize in albedo prediction.
To further enhance the robustness of decomposition results for subjects with significant domain gaps, a more effective approach may involve training the facial template on a more extensive and diverse set of subjects.

\begin{figure}[htbp]
    \centering
    \includegraphics[width=0.75\linewidth]{figs/supp/h3ds_v2.pdf}
    % \includegraphics[width=0.09\linewidth]{figs/supp/h3ds/nopre_render.png}\hspace{0pt}
    % \includegraphics[width=0.09\linewidth]{figs/supp/h3ds/nopre_diffuse.png}\hspace{0pt}
    % \includegraphics[width=0.09\linewidth]{figs/supp/h3ds/nopre_spec.png}\hspace{10pt}
    % \includegraphics[width=0.09\linewidth]{figs/supp/h3ds/nog_render.png}\hspace{0pt}
    % \includegraphics[width=0.09\linewidth]{figs/supp/h3ds/nog_diffuse.png}\hspace{0pt}
    % \includegraphics[width=0.09\linewidth]{figs/supp/h3ds/nog_spec.pdf}\hspace{10pt}
    % \includegraphics[width=0.09\linewidth]{figs/supp/h3ds/ours_render.png}\hspace{0pt}
    % \includegraphics[width=0.09\linewidth]{figs/supp/h3ds/ours_diffuse.png}\hspace{0pt}
    % \includegraphics[width=0.09\linewidth]{figs/supp/h3ds/ours_spec.png}
    % \\
    % \makebox[0.00\linewidth]{}\hspace{0pt}
    % % \makebox[0.19\linewidth]{\footnotesize\textbf{GT}}\hspace{5pt}
    % \makebox[0.3\linewidth]{\footnotesize\textbf{w/o $T_*$}}\hspace{5pt}
    % \makebox[0.3\linewidth]{\footnotesize\textbf{w/o $\mathcal{G}$}}\hspace{8pt}
    % \makebox[0.3\linewidth]{\footnotesize\textbf{Ours}}
    \caption{\textbf{Results on H3DS.} $T_*$ presents the facial template and $\mathcal{G}$ is the albedo gradient predictor. For each method showcased, the set of three images corresponds to rendering, diffuse, and specular, respectively.}
    \vspace{-10pt}
    \label{fig:h3ds}
\end{figure}

%This success could be attributed to the learnable albedo contribution weights from the template, initialized with relatively low values. Additionally, the prior knowledge of albedo distribution on faces could be transferred by the feature from the reflectance template. Nonetheless, to enhance the robustness of decomposition results for subjects with significant domain gaps, a more effective approach may involve training the face template on a more extensive and diverse set of subjects.

\section{Performance analysis}
\label{sec:analysis}
\textbf{Quantitative results.} We present the quantitative comparison results of all methods across different views in Tab.1 of the main text. Specifically, the evaluation of image synthesis quality is conducted using PSNR, SSIM, and LPIPS~\cite{zhang2018unreasonable} metrics. PSNR and SSIM only consider pixel-wise color differences between predictions and ground truth, which may not adequately reflect the synthesis reality. To evaluate the reality of rendered images, LPIPS uses a neural network to quantify perceptual similarity. In the 3-view setting, our method has a lower PSNR than DeformHead~\cite{xu2023deformable}. However, it excels over DeformHead in terms of LPIPS as it allows for the capture of more intricate appearance details, such as facial highlights and spots. Although the successful reconstruction of these details has little contribution to overall pixel-wise error metrics such as PSNR, it can enhance the realism of the rendered images.
% and PSNR may be influenced by large deviated color values in the poorly-covered regions of the training views. 

We use the Chamfer distance (CD) to evaluate the accuracy of geometry reconstruction. Compared to our method, geometry-oriented methods are more sensitive to geometry deformations, allowing them to capture intricate details such as teeth. However, the high sensitivity leads to false high-frequency geometry predictions, especially under sparse views. In Fig.4 of the main text and the figures in Sec.~\ref{sec:additional_results}, the facial skin appears smooth, but there are noticeable bumps in the predictions of VolSDF and DeformHead. Hence, our method has better performance in the CD metric under sparse view settings. 
In a low-view setting of 10 views, our method tackles a more complex decomposition task but still exhibits a comparable performance (marginally lower) to pure 3D reconstruction methods.
% Under a low-view setting of 10 views, our method exhibits a marginally lower performance compared to the 3D reconstruction task, primarily attributed to the heightened complexity of our decomposition task.

In Tab.3 of the main text, we present a quantitative comparison of decomposition quality between our method and NeuFace. Leveraging a general reflectance facial template, \textbf{SFDM} achieves robust decomposition of reflectance terms, leading to significantly superior diffuse and specular reflectance results compared to NeuFace. Specifically, NeuFace often contributes all reflectance to the diffuse term since the optimization simply relies on fitting facial images without reflectance supervision. Consequently, its specular decomposition performance deteriorates notably under sparse-view settings.

\begin{figure}[htbp]
    \vspace{0pt}
    \centering
    \includegraphics[width=0.9\linewidth]{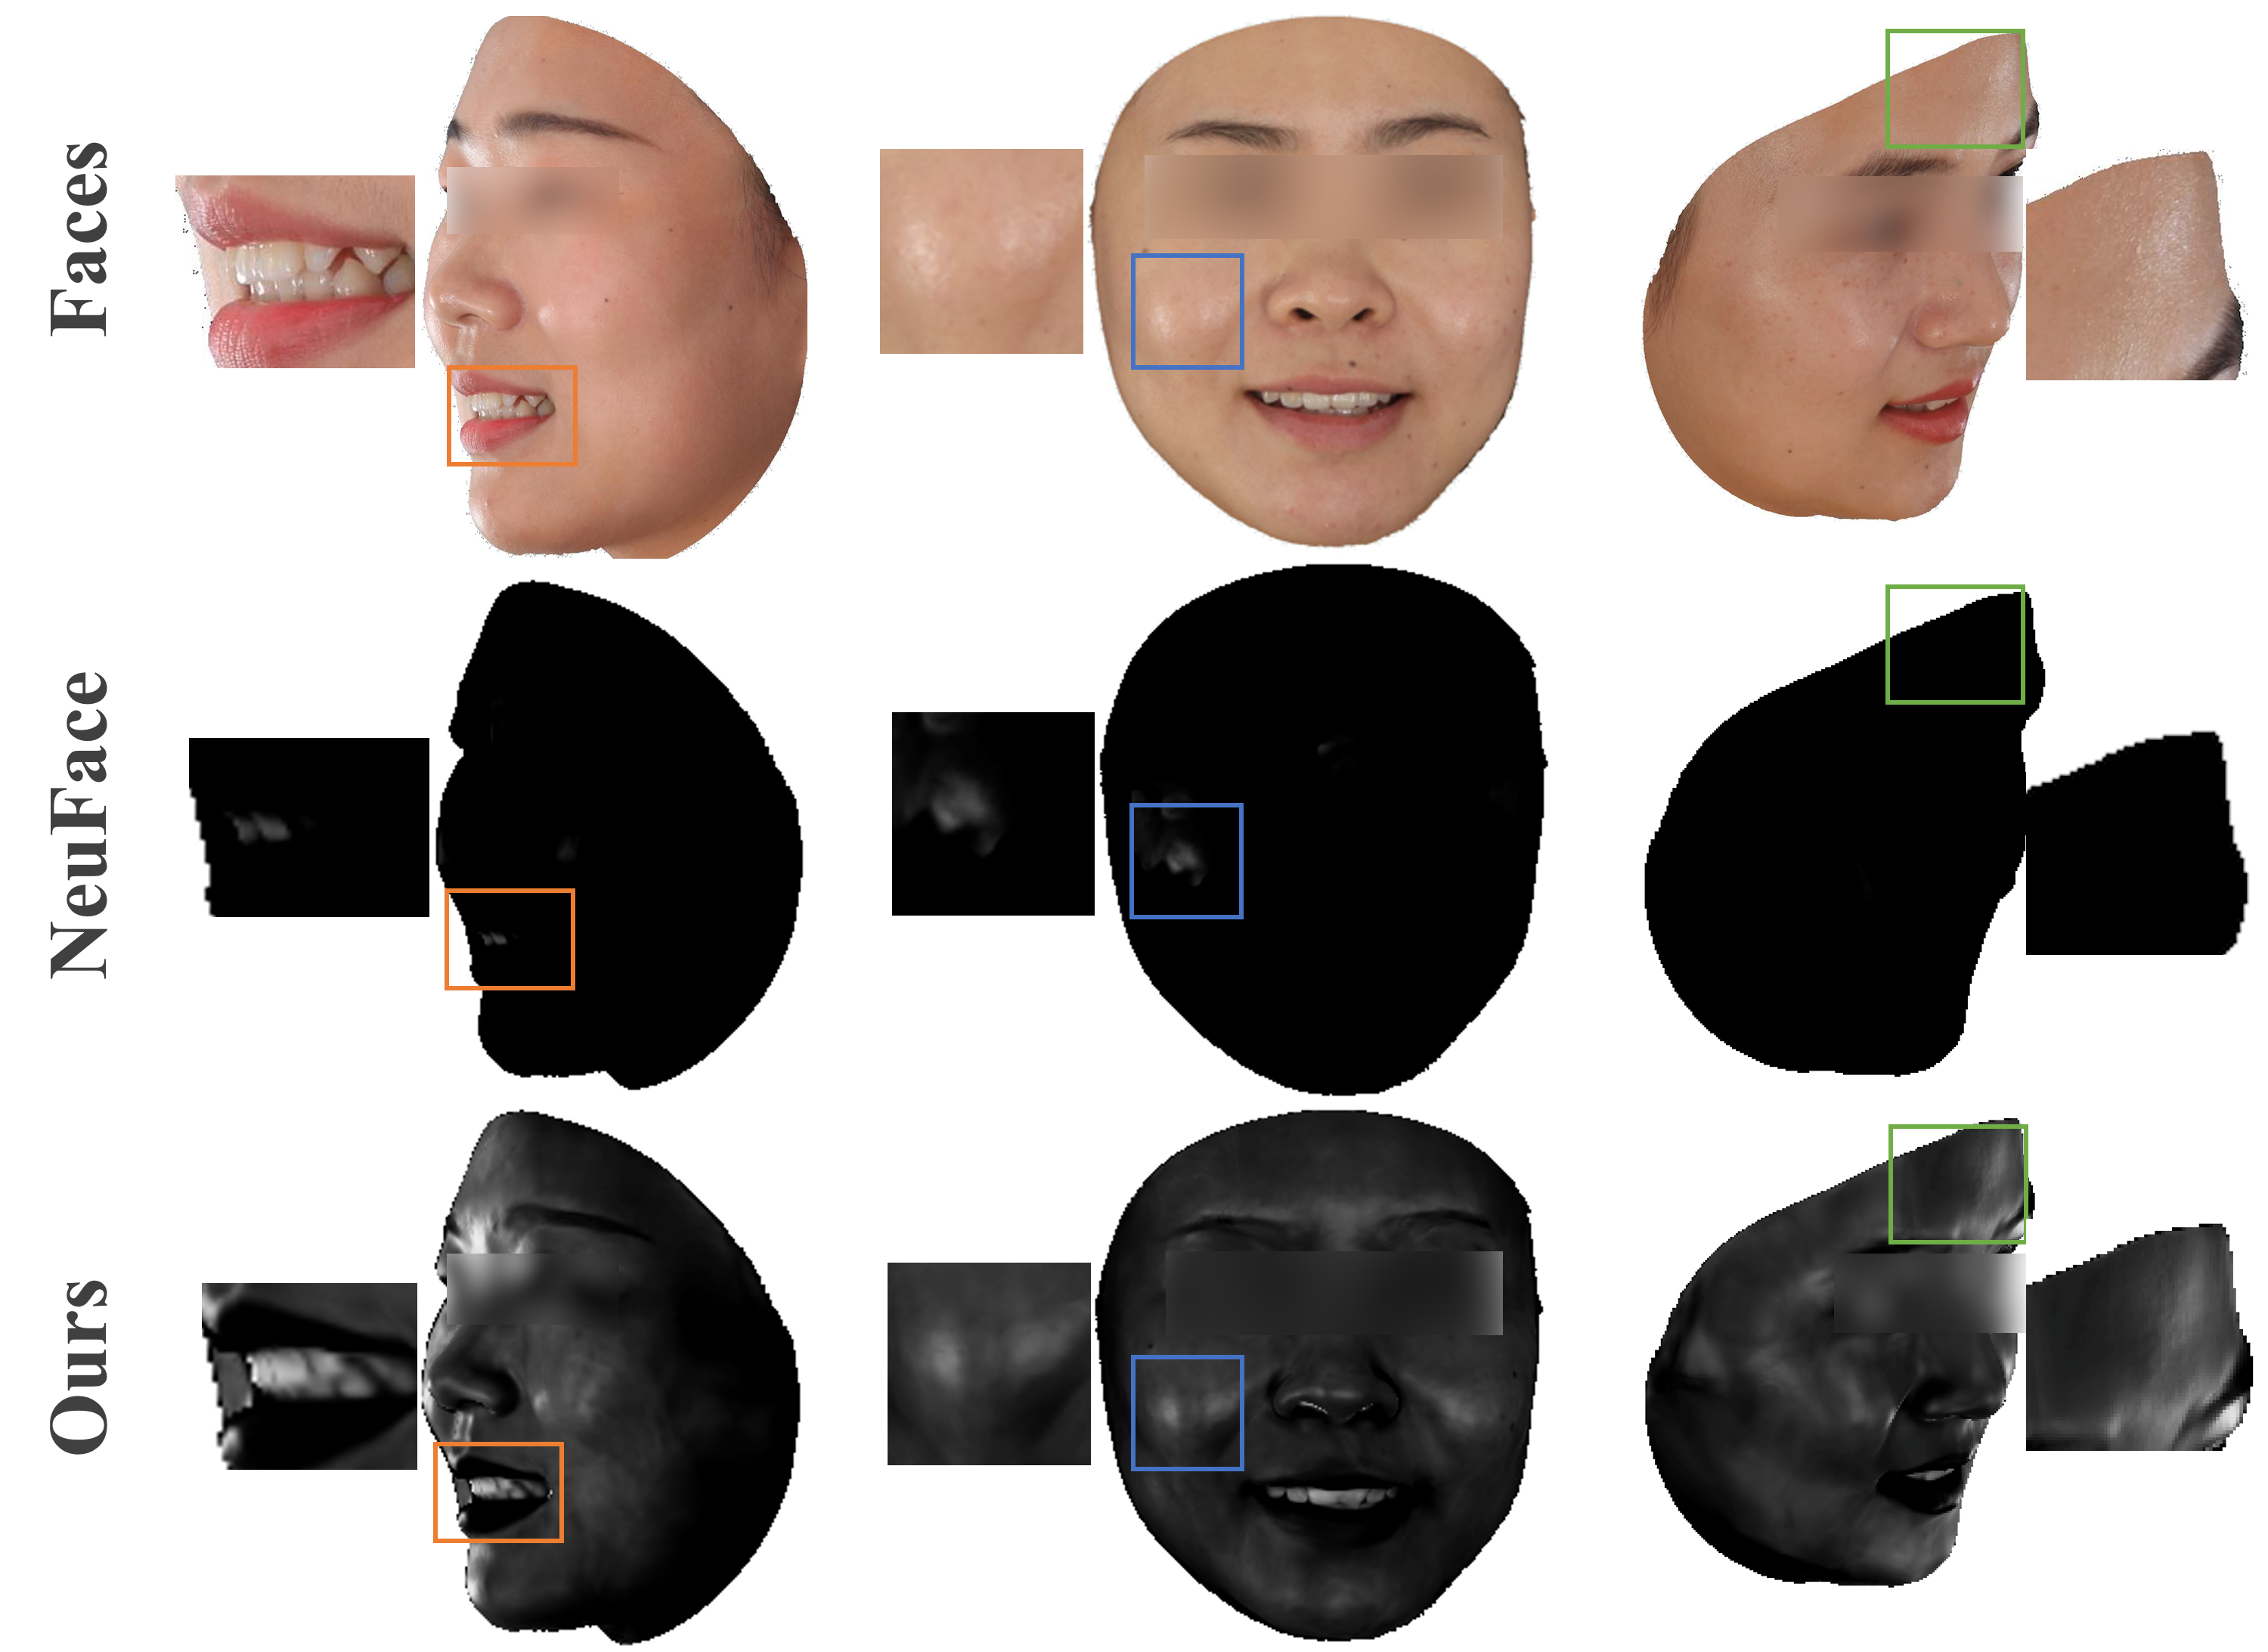}
    \vspace{-5pt}
    \caption{Comparison with NeuFace~\cite{zheng2023neuface} in terms of specular reflectance decomposition.}
    \label{fig:spec_cmp}
\end{figure}

\noindent\textbf{Qualitative results.} Our method outperforms other BRDF decomposition methods in terms of all metrics, demonstrating superior rendering and geometry reconstruction effects. Besides, as shown in Fig.~\ref{fig:spec_cmp} and Sec.~\ref{sec:additional_results}, our method can robustly decompose specular terms across various subjects and settings, benefiting from the comprehensive prior knowledge of the learned facial template. Considering that there is no ground truth for specular reflectance, we introduce a straightforward metric called specular failure rate, representing the percentage of entirely empty specular output. This metric facilitates a quantitative comparison between our method and NeuFace. According to the statistics, our method achieves a specular failure rate of 0\%, whereas NeuFace's specular failure rates are 30\%, 25\%, and 20\% under 3 views, 5 views, and 10 views, respectively.

Furthermore, we observe that the TensoIR~\cite{jin2023tensoir} exhibits noticeable lining effects, prompting us to investigate. We find these effects are caused by sparse view conditions. When we utilize all training views, these phenomena disappear.

\begin{table*}[htbp]

\centering

\resizebox{0.8\linewidth}{!}{\begin{tabular}{l|c|c|c|c|c}
\hline
\textbf{Method}  & \textbf{Geometry} & \textbf{Reflectance} & \textbf{\# views} & \textbf{Fine Details} & \textbf{Requring Albedo GT} \\
\hline
\hline
\textbf{NeRF~\cite{mildenhall2021nerf}} & N & N & 20+ & Y & N\\
\textbf{VolSDF~\cite{yariv2021volume}} & Y & N & 20+ & Y & N\\
\textbf{DeformHead~\cite{xu2023deformable}} & Y & N & 10 & Y & N \\
\textbf{TensoIR~\cite{jin2023tensoir}} & Y & Y & 20+ & Y & N \\
\textbf{NeuFace~\cite{zheng2023neuface}} & Y & Y & 20+ & Y & N \\
\textbf{AlbedoMM~\cite{smith2020morphable}} & Y & Y & 1 & N & Y \\
\textbf{TRUST~\cite{feng2022towards}} & Y & Y & 1 & N & Y \\
\textbf{Relightify~\cite{chen2022relighting4d}} & Y & Y & 1 & N & Y \\
\textbf{Fitme~\cite{lattas2023fitme}} & Y & Y & 1 & N & Y \\
\textbf{RefMM~\cite{han2023learning}} & Y & Y & 1 & N & N \\
\hline
\textbf{Ours}  & Y & Y & 3 & Y & N \\
\hline
\end{tabular}}

\caption{\textbf{Qualitative comparison with other methods.} We assess the capabilities of various methods in comparison to our own. Our approach can achieve detailed decomposition and reconstruction from three-view images, without the need for intricate lighting and ground truth albedo prerequisites.}

\label{tab:func_cmp}
\end{table*}

\section{Discussion with single-view methods}
\label{sec:single}

Our method focuses on the reconstruction from sparse views, and thus we do not discuss single-view methods in detail in the main text. However, this section will discuss our relationship with single-view approaches. Although sparse views offer limited perspectives, they can still provide rich 3D information when combined with camera angles. For instance, with at least two-view images, the 3D coordinates of a point corresponding in real space across both views can be calculated using its 2D coordinates and camera parameters. Conversely, single-view images contain only 2D information and lack 3D details, often relying on 3D estimation methods for reconstruction. Due to the limited information in a single 2D image, single-view approaches typically require extensive training data (1000+ images) across a wide variety of identities to obtain the ability to perform 3D estimation effectively. By contrast, multi-view methods can extract vast quantities of 3D information from images of a single identity, making them more efficient for tasks where multiple views are available.

One type of single-view approach involves GAN-based methods, such as EG3D~\cite{chan2022efficient_eg3d}, which trains models to generate 3D meshes and novel view images with extensive training data. However, this method faces challenges with data volume requirements and consistency issues in generated images (e.g., eyes looking towards the camera from all views). Similarly, Relightify~\cite{papantoniou2023relightify} employs another generative method, the diffusion model, which also requires a large number of training images.

Another approach is based on parametric face models, predicting facial parameters from a single-view image to reconstruct faces. For example, AlbedoMM~\cite{smith2020morphable} uses 3DMM~\cite{blanz2023morphable}, TRUST~\cite{feng2022towards} is based on FLAME~\cite{li2017learning_flame}, and RefMM~\cite{han2023learning} utilizes BFM09~\cite{paysan20093d_bfm09}. However, due to the difficulty of face decomposition tasks, these methods often require higher quality training data, such as various environmental lighting settings (3D-RFE dataset~\cite{stratou2011effect} in AlbedoMM) and pseudo ground truth reflectance (utilizing texture maps in TRUST and diffuse maps in the 3D-RFE dataset). Additionally, the use of 3D morphable face models, while efficient in compressing facial expressions, tends to lose many details in face reconstruction. As shown in Fig.~\ref{fig:refmm}, our experiments with RefMM's reconstruction results, although capable of generating geometry and reflectance from a single view, significantly lack the facial details and realism achieved by our SFDM.

\begin{figure}[htbp]
    \vspace{0pt}
    \centering
    \includegraphics[width=0.9\linewidth]{figs/supp/refmm.pdf}
    \vspace{-5pt}
    \caption{\textbf{Comparison with RefMM.} The first column presents the ground truth images, while the second column showcases our reconstruction results. Regarding RefMM's outcomes, from left to right, the sequence includes the reconstruction result, diffuse shading, specular shading, and geometry.}
    \label{fig:refmm}
\end{figure}

\section{Ethnic statement}
\label{sec:ethnic}

Our method is primarily used for facial reconstruction, thus necessitating a focus on protecting individuals' privacy. We utilized the \textit{Facescape} dataset, of which only a subset of IDs are publishable. Consequently, we applied mosaic processing (approved by the publishers of \textit{Facescape}) to all portraits not on the publishable list, similar to what is done in Sec.~\ref{sec:additional_results}, to safeguard personal privacy. We encourage future SFDM users to conduct facial reconstruction and decomposition using facial images for which they have obtained authorization, thereby respecting people's portrait rights.
 
\section{Additional results}
\label{sec:additional_results}

Here we provide more results to illustrate the effectiveness of our method. Fig.~\ref{fig:3view-sub12} - \ref{fig:3view-sub342}, Fig.~\ref{fig:5view-sub12} - \ref{fig:5view-sub342}, Fig.~\ref{fig:10view-sub13} - \ref{fig:10view-sub344} are results under 3-view settings, 5-view settings, and 10-view (low-view) settings, respectively. Specifically, the rendering results are calibrated as Sec.~\ref{sec:implementation}, correcting the overall color deviations, such as the results of NeuFace~\cite{zheng2023neuface} in Fig.~\ref{fig:3view-sub12}. In the \textit{Facescape} dataset, only four subjects (122, 212, 340, 344) are cleared for publication. For the remaining subjects, we have applied the mosaic technique to ensure their anonymity.
