# Supplementary material for: SFDM: Robust Decomposition of Geometry and Reflectance for Realistic Face Rendering from Sparse-view Images
Source: arXiv:2312.06085 source file (2025-03-15)
Supplement: Supplementary file 13 [file fig_3view_16.tex]

\begin{figure*}[!t]
    \centering
    % \makebox[0.01\linewidth]{}\hspace{0.1cm}
    \hspace{8pt}\makebox[0.1\linewidth]{VolSDF}\hspace{12pt}
    \makebox[0.1\linewidth]{DeformHead}\hspace{8pt}
    \makebox[0.1\linewidth]{PhySG}\hspace{8pt}
    \makebox[0.1\linewidth]{TensoIR}\hspace{8pt}
    \makebox[0.1\linewidth]{NeuFace}\hspace{8pt}
    \makebox[0.1\linewidth]{Ours}\hspace{8pt}
    \makebox[0.1\linewidth]{GT}
    \\
    \makebox[0.02\linewidth]{\rotatebox{90}{\hspace{0pt}\textbf{Rendering}}}\hspace{5pt}
    \includegraphics[clip, width=0.1\linewidth]{figs/supp/3view/16/volsdf_render.pdf}\hspace{8pt}
    \includegraphics[clip,width=0.1\linewidth]{figs/supp/3view/16/deform_render.pdf}\hspace{8pt}
    \includegraphics[clip,width=0.1\linewidth]{figs/supp/3view/16/physg_render.pdf}\hspace{8pt}
    \includegraphics[clip,width=0.1\linewidth]{figs/supp/3view/16/tensoir_render.pdf}\hspace{8pt}
    \includegraphics[clip, width=0.1\linewidth]{figs/supp/3view/16/neuface_render.pdf}\hspace{8pt}
    \includegraphics[clip, width=0.1\linewidth]{figs/supp/3view/16/ours_render.pdf}
    \hspace{8pt}
    \includegraphics[clip, width=0.1\linewidth]{figs/supp/3view/16/gt_16.pdf}
    \vspace{5pt}
    \\
    \makebox[0.02\linewidth]{\rotatebox{90}{\hspace{5pt}\textbf{Normal}}}\hspace{5pt}
    \includegraphics[clip, width=0.1\linewidth]{figs/supp/3view/16/volsdf_normal.pdf}\hspace{8pt}
    \includegraphics[clip,width=0.1\linewidth]{figs/supp/3view/16/deform_normal.pdf}\hspace{8pt}
    \includegraphics[clip,width=0.1\linewidth]{figs/supp/3view/16/physg_normal.pdf}\hspace{8pt}
    \includegraphics[clip,width=0.1\linewidth]{figs/supp/3view/16/tensoir_normal.pdf}\hspace{8pt}
    \includegraphics[clip, width=0.1\linewidth]{figs/supp/3view/16/neuface_normal.pdf}\hspace{8pt}
    \includegraphics[clip, width=0.1\linewidth]{figs/supp/3view/16/ours_normal.pdf}
    \hspace{8pt}
    \includegraphics[clip, width=0.1\linewidth]{figs/supp/3view/16/gt_16_mesh.jpg}
    \vspace{5pt}
    \\
    \makebox[0.02\linewidth]{\rotatebox{90}{\hspace{10pt}\textbf{Diffuse}}}\hspace{5pt}
    \includegraphics[clip, width=0.1\linewidth]{figs/supp/na.jpg}\hspace{8pt}
    \includegraphics[clip, width=0.1\linewidth]{figs/supp/na.jpg}\hspace{8pt}
    \includegraphics[clip,width=0.1\linewidth]{figs/supp/3view/16/physg_diffuse.pdf}\hspace{8pt}
    \includegraphics[clip,width=0.1\linewidth]{figs/supp/3view/16/tensoir_diffuse.pdf}\hspace{8pt}
    \includegraphics[clip, width=0.1\linewidth]{figs/supp/3view/16/neuface_diffuse.pdf}\hspace{8pt}
    \includegraphics[clip, width=0.1\linewidth]{figs/supp/3view/16/ours_diffuse.pdf}
    \hspace{8pt}
    \makebox[0.1\linewidth]{}
    \vspace{5pt}
    \\
    \makebox[0.02\linewidth]{\rotatebox{90}{\hspace{8pt}\textbf{Specular}}}\hspace{5pt}
    \includegraphics[clip, width=0.1\linewidth]{figs/supp/na.jpg}\hspace{8pt}
    \includegraphics[clip, width=0.1\linewidth]{figs/supp/na.jpg}\hspace{8pt}
    \includegraphics[clip,width=0.1\linewidth]{figs/supp/3view/16/physg_spec.pdf}\hspace{8pt}
    \includegraphics[clip,width=0.1\linewidth]{figs/supp/3view/16/tensoir_spec.pdf}\hspace{8pt}
    \includegraphics[clip, width=0.1\linewidth]{figs/supp/3view/16/neuface_spec.pdf}\hspace{8pt}
    \includegraphics[clip, width=0.1\linewidth]{figs/supp/3view/16/ours_spec.pdf}
    \hspace{8pt}
    \makebox[0.1\linewidth]{}
    \vspace{5pt}

    \caption{Comparison under a 3-view setting for Subject 16.}
    \label{fig:3view-sub16}
\end{figure*}
