# Supplementary material for: SFDM: Robust Decomposition of Geometry and Reflectance for Realistic Face Rendering from Sparse-view Images
Source: arXiv:2312.06085 source file (2025-03-15)
Supplement: Supplementary file 27 [file age.tex]

\begin{figure}[htbp]
    % \vspace{-10pt}
    \centering
    \makebox[0.02\linewidth]{\rotatebox{90}{\hspace{15pt}\footnotesize 17 Grin}}\hspace{5pt}
    \includegraphics[width=0.15\linewidth]{figs/supp/age/17/17_render.pdf}\hspace{5pt}
    \includegraphics[width=0.15\linewidth]{figs/supp/age/17/17_normal.pdf}\hspace{5pt}
    \includegraphics[width=0.15\linewidth]{figs/supp/age/17/17_diffuse.pdf}\hspace{5pt}
    \includegraphics[width=0.15\linewidth]{figs/supp/age/17/17_spec.pdf}
    \\
    \makebox[0.02\linewidth]{\rotatebox{90}{\hspace{12pt}\footnotesize 14 Grin}}\hspace{5pt}
    \includegraphics[width=0.15\linewidth]{figs/supp/age/14/14_render.pdf}\hspace{5pt}
    \includegraphics[width=0.15\linewidth]{figs/supp/age/14/14_normal.pdf}\hspace{5pt}
    \includegraphics[width=0.15\linewidth]{figs/supp/age/14/14_diffuse.pdf}\hspace{5pt}
    \includegraphics[width=0.15\linewidth]{figs/supp/age/14/14_spec.pdf}
    \\
    \makebox[0.02\linewidth]{}\hspace{5pt}
    % \makebox[0.15\linewidth]{\footnotesize\textbf{GT}}\hspace{5pt}
    \makebox[0.15\linewidth]{\footnotesize\textbf{Rendering}}\hspace{5pt}
    \makebox[0.15\linewidth]{\footnotesize\textbf{Normal}}\hspace{5pt}
    \makebox[0.15\linewidth]{\footnotesize\textbf{Diffuse}}\hspace{5pt}
    \makebox[0.15\linewidth]{\footnotesize\textbf{Specular}}\hspace{5pt}
    \caption{Results of subjects with large variations of skin colors and ages from the template.}
    % \vspace{-10pt}
    \label{fig:age}
\end{figure}
