# Supplementary material for: SFDM: Robust Decomposition of Geometry and Reflectance for Realistic Face Rendering from Sparse-view Images
Source: arXiv:2312.06085 source file (2025-03-15)
Supplement: Supplementary file 28 [file expression.tex]

\begin{figure}[htbp]
    \centering
    \makebox[0.02\linewidth]{\rotatebox{90}{\hspace{15pt}\footnotesize 212 Grin}}\hspace{5pt}
    \includegraphics[width=0.15\linewidth]{figs/supp/expression/212_16/212_16_render.pdf}\hspace{5pt}
    \includegraphics[width=0.15\linewidth]{figs/supp/expression/212_16/212_16_normal.pdf}\hspace{5pt}
    \includegraphics[width=0.15\linewidth]{figs/supp/expression/212_16/212_16_diffuse.pdf}\hspace{5pt}
    \includegraphics[width=0.15\linewidth]{figs/supp/expression/212_16/212_16_spec.pdf}
    \\
    \makebox[0.02\linewidth]{\rotatebox{90}{\hspace{12pt}\footnotesize 212 Smile}}\hspace{5pt}
    \includegraphics[width=0.15\linewidth]{figs/supp/expression/212_2/212_2_render.pdf}\hspace{5pt}
    \includegraphics[width=0.15\linewidth]{figs/supp/expression/212_2/212_2_normal.pdf}\hspace{5pt}
    \includegraphics[width=0.15\linewidth]{figs/supp/expression/212_2/212_2_diffuse.pdf}\hspace{5pt}
    \includegraphics[width=0.15\linewidth]{figs/supp/expression/212_2/212_2_spec.pdf}
    \\
    \makebox[0.02\linewidth]{\rotatebox{90}{\hspace{15pt}\footnotesize 344 Grin}}\hspace{5pt}
    \includegraphics[width=0.15\linewidth]{figs/supp/expression/344_16/render.pdf}\hspace{5pt}
    \includegraphics[width=0.15\linewidth]{figs/supp/expression/344_16/normal.pdf}\hspace{5pt}
    \includegraphics[width=0.15\linewidth]{figs/supp/expression/344_16/diffuse.pdf}\hspace{5pt}
    \includegraphics[width=0.15\linewidth]{figs/supp/expression/344_16/spec.pdf}
    \\
    \makebox[0.02\linewidth]{\rotatebox{90}{\hspace{12pt}\footnotesize 344 Angry}}\hspace{5pt}
    \includegraphics[width=0.15\linewidth]{figs/supp/expression/344_4/render.pdf}\hspace{5pt}
    \includegraphics[width=0.15\linewidth]{figs/supp/expression/344_4/normal.pdf}\hspace{5pt}
    \includegraphics[width=0.15\linewidth]{figs/supp/expression/344_4/diffuse.pdf}\hspace{5pt}
    \includegraphics[width=0.15\linewidth]{figs/supp/expression/344_4/spec.pdf}
    \\
    \makebox[0.02\linewidth]{}\hspace{5pt}
    % \makebox[0.15\linewidth]{\footnotesize\textbf{GT}}\hspace{5pt}
    \makebox[0.15\linewidth]{\footnotesize\textbf{Rendering}}\hspace{5pt}
    \makebox[0.15\linewidth]{\footnotesize\textbf{Normal}}\hspace{5pt}
    \makebox[0.15\linewidth]{\footnotesize\textbf{Diffuse}}\hspace{5pt}
    \makebox[0.15\linewidth]{\footnotesize\textbf{Specular}}\hspace{5pt}
    \caption{Results on different expressions.}
    \vspace{-10pt}
    \label{fig:expressions}
\end{figure}
