# Supplementary material for: SFDM: Robust Decomposition of Geometry and Reflectance for Realistic Face Rendering from Sparse-view Images
Source: arXiv:2312.06085 source file (2025-03-15)
Supplement: Supplementary file 29 [file h3ds.tex]

\begin{figure}[htbp]
    \centering
    \includegraphics[width=0.75\linewidth]{figs/supp/h3ds_v2.pdf}
    % \includegraphics[width=0.09\linewidth]{figs/supp/h3ds/nopre_render.png}\hspace{0pt}
    % \includegraphics[width=0.09\linewidth]{figs/supp/h3ds/nopre_diffuse.png}\hspace{0pt}
    % \includegraphics[width=0.09\linewidth]{figs/supp/h3ds/nopre_spec.png}\hspace{10pt}
    % \includegraphics[width=0.09\linewidth]{figs/supp/h3ds/nog_render.png}\hspace{0pt}
    % \includegraphics[width=0.09\linewidth]{figs/supp/h3ds/nog_diffuse.png}\hspace{0pt}
    % \includegraphics[width=0.09\linewidth]{figs/supp/h3ds/nog_spec.pdf}\hspace{10pt}
    % \includegraphics[width=0.09\linewidth]{figs/supp/h3ds/ours_render.png}\hspace{0pt}
    % \includegraphics[width=0.09\linewidth]{figs/supp/h3ds/ours_diffuse.png}\hspace{0pt}
    % \includegraphics[width=0.09\linewidth]{figs/supp/h3ds/ours_spec.png}
    % \\
    % \makebox[0.00\linewidth]{}\hspace{0pt}
    % % \makebox[0.19\linewidth]{\footnotesize\textbf{GT}}\hspace{5pt}
    % \makebox[0.3\linewidth]{\footnotesize\textbf{w/o $T_*$}}\hspace{5pt}
    % \makebox[0.3\linewidth]{\footnotesize\textbf{w/o $\mathcal{G}$}}\hspace{8pt}
    % \makebox[0.3\linewidth]{\footnotesize\textbf{Ours}}
    \caption{\textbf{Results on H3DS.} $T_*$ presents the facial template and $\mathcal{G}$ is the albedo gradient predictor. For each method showcased, the set of three images corresponds to rendering, diffuse, and specular, respectively.}
    \vspace{-10pt}
    \label{fig:h3ds}
\end{figure}
