# Supplementary material for: SFDM: Robust Decomposition of Geometry and Reflectance for Realistic Face Rendering from Sparse-view Images
Source: arXiv:2312.06085 source file (2025-03-15)
Supplement: Supplementary file 30 [file h3ds_old.tex]

\begin{figure}[htbp]
    \centering
    \makebox[0.02\linewidth]{\rotatebox{90}{\hspace{15pt}\footnotesize w/o $T_{*}$}}\hspace{5pt}
    % \includegraphics[width=0.19\linewidth]{example-image}\hspace{5pt}
    \includegraphics[width=0.13\linewidth]{figs/supp/h3ds/nopre_render.png}\hspace{5pt}
    \includegraphics[width=0.13\linewidth]{figs/supp/h3ds/nopre_normal.png}\hspace{5pt}
    \includegraphics[width=0.13\linewidth]{figs/supp/h3ds/nopre_diffuse.png}\hspace{5pt}
    \includegraphics[width=0.13\linewidth]{figs/supp/h3ds/nopre_spec.png}
    \\
    \makebox[0.02\linewidth]{\rotatebox{90}{\hspace{15pt}\footnotesize w/o $\mathcal{G}$}}\hspace{5pt}
    % \includegraphics[width=0.19\linewidth]{example-image}\hspace{5pt}
    \includegraphics[width=0.13\linewidth]{figs/supp/h3ds/nog_render.png}\hspace{5pt}
    \includegraphics[width=0.13\linewidth]{figs/supp/h3ds/nog_normal.pdf}\hspace{5pt}
    \includegraphics[width=0.13\linewidth]{figs/supp/h3ds/nog_diffuse.png}\hspace{5pt}
    \includegraphics[width=0.13\linewidth]{figs/supp/h3ds/nog_spec.pdf}
    \\
    \makebox[0.02\linewidth]{\rotatebox{90}{\hspace{15pt}\footnotesize Ours}}\hspace{5pt}
    % \includegraphics[width=0.19\linewidth]{example-image}\hspace{5pt}
    \includegraphics[width=0.13\linewidth]{figs/supp/h3ds/ours_render.png}\hspace{5pt}
    \includegraphics[width=0.13\linewidth]{figs/supp/h3ds/ours_normal.png}\hspace{5pt}
    \includegraphics[width=0.13\linewidth]{figs/supp/h3ds/ours_diffuse.png}\hspace{5pt}
    \includegraphics[width=0.13\linewidth]{figs/supp/h3ds/ours_spec.png}
    \\
    \makebox[0.02\linewidth]{}\hspace{5pt}
    % \makebox[0.19\linewidth]{\footnotesize\textbf{GT}}\hspace{5pt}
    \makebox[0.13\linewidth]{\footnotesize\textbf{Rendering}}\hspace{5pt}
    \makebox[0.13\linewidth]{\footnotesize\textbf{Normal}}\hspace{5pt}
    \makebox[0.13\linewidth]{\footnotesize\textbf{Diffuse}}\hspace{5pt}
    \makebox[0.13\linewidth]{\footnotesize\textbf{Specular}}\hspace{5pt}
    \caption{\textbf{Results on H3DS.} The first row presents the results of SFDM without the facial template, and the second row shows the results of SFDF without the albedo gradient predictor.}
    \vspace{-10pt}
    \label{fig:h3ds}
\end{figure}
